# Supplementary material for: Full-spectrum modeling of mobile gamma-ray spectrometry systems in scattering media
Source: arXiv:2506.17820 ancillary file (2025-12-20)
Supplement: Supplementary file 1 [file Supplementary_Materials.pdf]

# Supplementary Information for

## Full-spectrum modeling of mobile gamma-ray spectrometry systems in scattering media

David Breitenmoser<sup>1,2,\*</sup>, Alberto Stabilini<sup>1</sup>, Sabine Mayer<sup>1</sup>

<sup>1</sup>Department of Radiation Safety and Security, Paul Scherrer Institute (PSI), Forschungsstrasse 111, Villigen PSI, 5232, Switzerland

<sup>2</sup>Department of Nuclear Engineering & Radiological Sciences, University of Michigan, 2355 Bonisteel Blvd., Ann Arbor, MI 48109-2104, United States of America

\*Lead and contact author: David Breitenmoser (E-Mail: david.breitenmoser@psi.ch, ORCID: 0000-0003-0339-6592)

### The PDF includes:

Supplementary Figures S1–S13

Supplementary References

# Contents

|                                      |             |
|--------------------------------------|-------------|
| <b>List of Supplementary Figures</b> | <b>SIII</b> |
| <b>S1 Supplementary Figures</b>      | <b>S1</b>   |
| <b>Supplementary References</b>      | <b>S14</b>  |

## List of Supplementary Figures

|     |                                                                                                                                                                 |     |
|-----|-----------------------------------------------------------------------------------------------------------------------------------------------------------------|-----|
| S1  | Plane wave source radius sensitivity analysis . . . . .                                                                                                         | S1  |
| S2  | Double-differential gamma-ray flux bank . . . . .                                                                                                               | S2  |
| S3  | Angular dispersion of the SAGRS system's instrument response at $E_\gamma = 88$ keV . . . . .                                                                   | S3  |
| S4  | Angular dispersion of the SAGRS system's instrument response at $E_\gamma = 2615$ keV . . . . .                                                                 | S4  |
| S5  | Combined statistical and and systematic uncertainties in the spectral dispersion of the SAGRS system's instrument response . . . . .                            | S5  |
| S6  | Combined statistical and and systematic uncertainties in the angular dispersion of the SAGRS system's instrument response at $E_\gamma = 88$ keV . . . . .      | S6  |
| S7  | Combined statistical and and systematic uncertainties in the angular dispersion of the SAGRS system's instrument response at $E_\gamma = 662$ keV . . . . .     | S7  |
| S8  | Combined statistical and and systematic uncertainties in the angular dispersion of the SAGRS system's instrument response at $E_\gamma = 2615$ keV . . . . .    | S8  |
| S9  | Relative deviation in the angular dispersion of the SAGRS system's instrument response for selected state variable changes at $E_\gamma = 88$ keV . . . . .     | S9  |
| S10 | Relative deviation in the angular dispersion of the SAGRS system's instrument response for selected state variable changes at $E_\gamma = 2615$ keV . . . . .   | S10 |
| S11 | Relative deviation in the angular dispersion of the SAGRS system's instrument response for additional state variable changes at $E_\gamma = 88$ keV . . . . .   | S11 |
| S12 | Relative deviation in the angular dispersion of the SAGRS system's instrument response for additional state variable changes at $E_\gamma = 662$ keV . . . . .  | S12 |
| S13 | Relative deviation in the angular dispersion of the SAGRS system's instrument response for additional state variable changes at $E_\gamma = 2615$ keV . . . . . | S13 |

## S1 Supplementary Figures

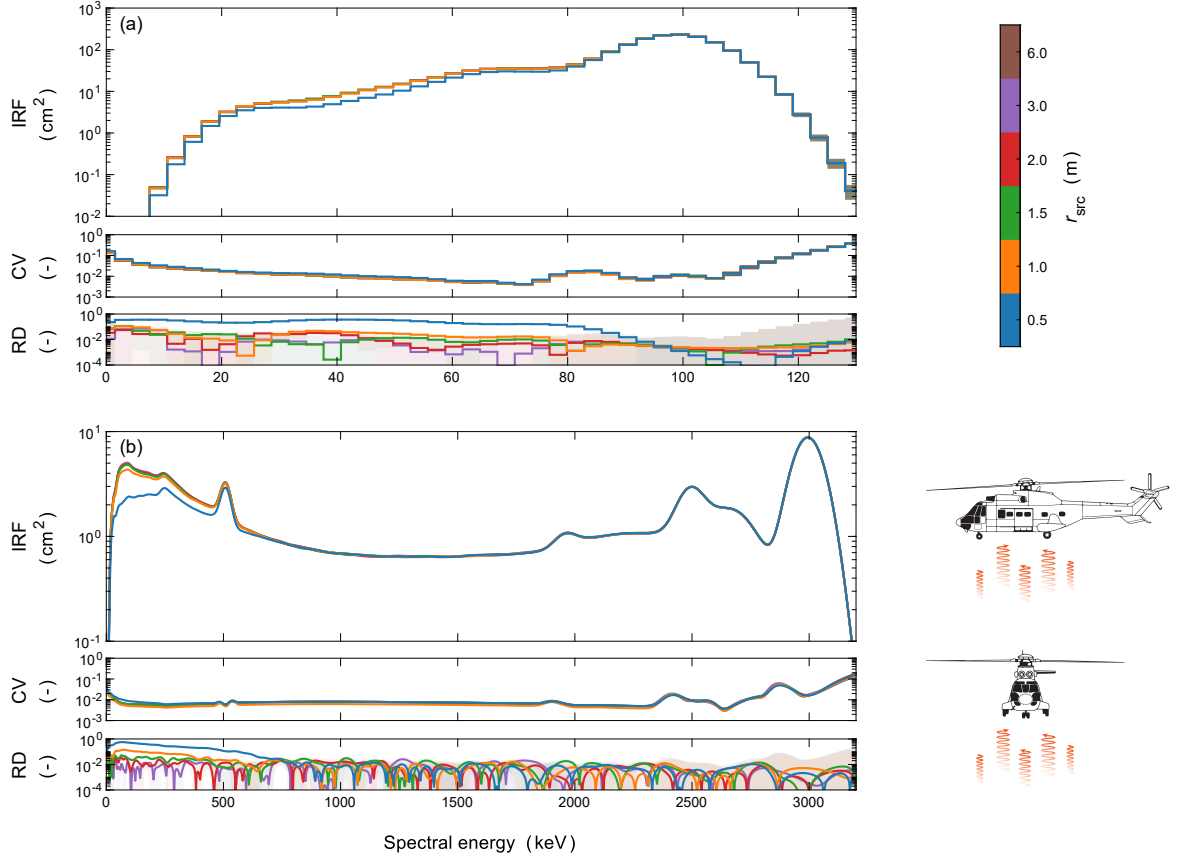

**Figure S1** Here, we present the results of a sensitivity study conducted to assess the effect of the source radius  $r_{\text{src}}$  on the simulated instrument response function (IRF). For that purpose, we evaluated the IRF by a circular monoenergetic gamma-ray plane wave with varying source radius  $r_{\text{src}}$  oriented along the normal axis  $z'$  (cf. Fig. 1 in the main study). This specific direction shows the largest effective instrument response in the Compton band  $\mathcal{B}_C$  (cf. Sec. IV in the main study). The associated Monte Carlo simulations were repeated for two gamma-ray energies: (A)  $E_\gamma = 100 \text{ keV}$ . (b)  $E_\gamma = 3000 \text{ keV}$ . For each energy, the simulated mean instrument response  $R$  is displayed as a function of the spectral energy  $E'$  with a constant spectral energy bin width  $\Delta E' \sim 3 \text{ keV}$ . Uncertainties are provided as 1 standard error shaded areas. In addition, the coefficient of variation (CV) as well as the relative deviation (RD) with respect to the instrument response at the bounding radius  $r_{\text{src}} = 6 \text{ m}$  are displayed. The displayed line drawings of the AS332M1 helicopter were adapted from Jetijones, CC BY 3.0, via Wikimedia Commons.

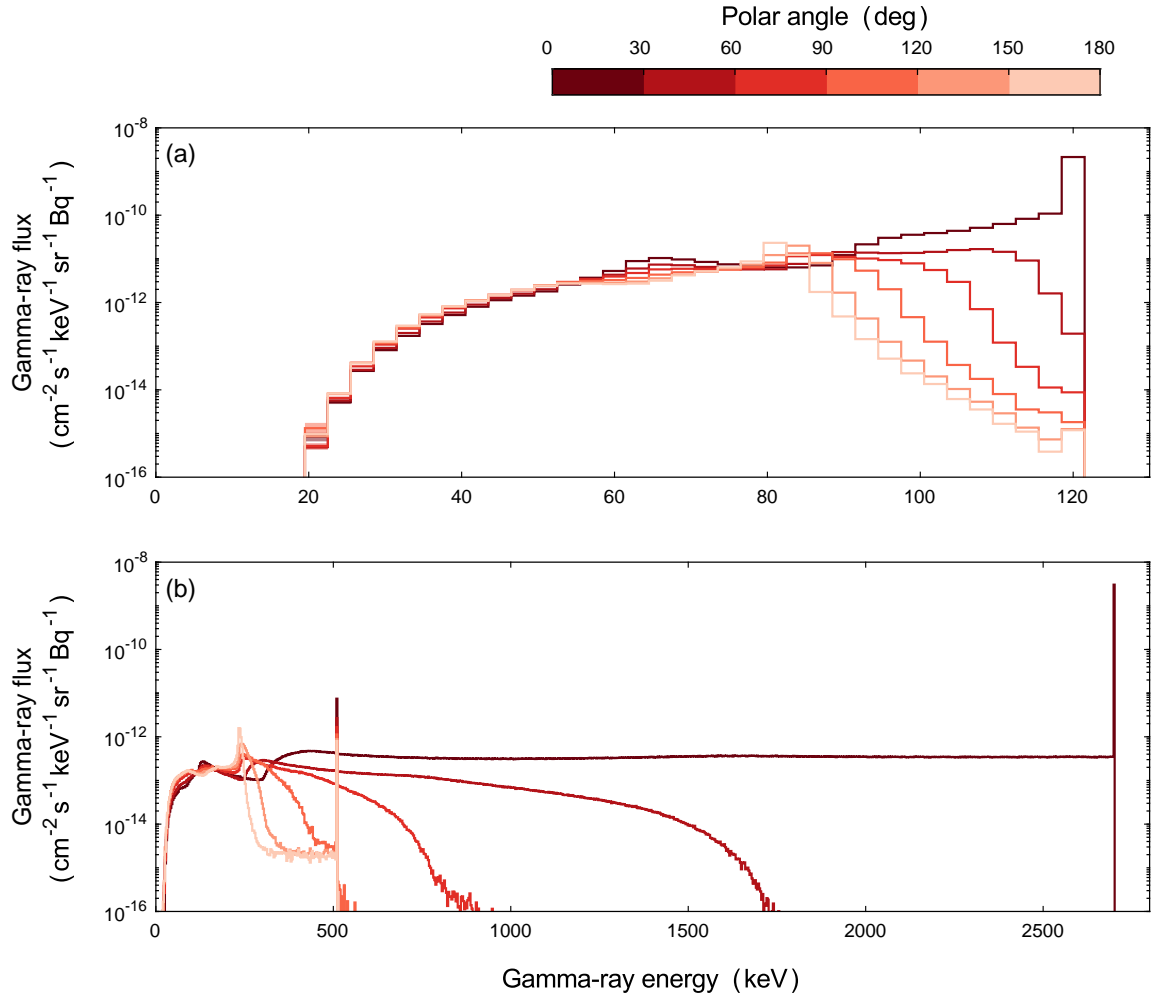

**Figure S2** Here, we display signatures from the double-differential gamma-ray flux bank generated for the benchmark verification in the main study (see Section IV C). As described in detail in Section III B in the main study, we evaluated the double differential gamma-ray flux for two monoenergetic isotropic gamma-ray point sources with energies: (a) 120 keV. (b) 2.7 MeV. In each subfigure, the mean double-differential gamma-ray flux signatures are displayed as a function of the gamma-ray energy  $E_\gamma$  and the polar angle  $\varphi$  with respect to the line-of-sight axis between the source and the reference scoring area. Uncertainties are provided as 1 standard error shaded areas. For visualization purposes, the signatures were rebinned from a  $5^\circ$  to a  $30^\circ$  polar angle spacing.

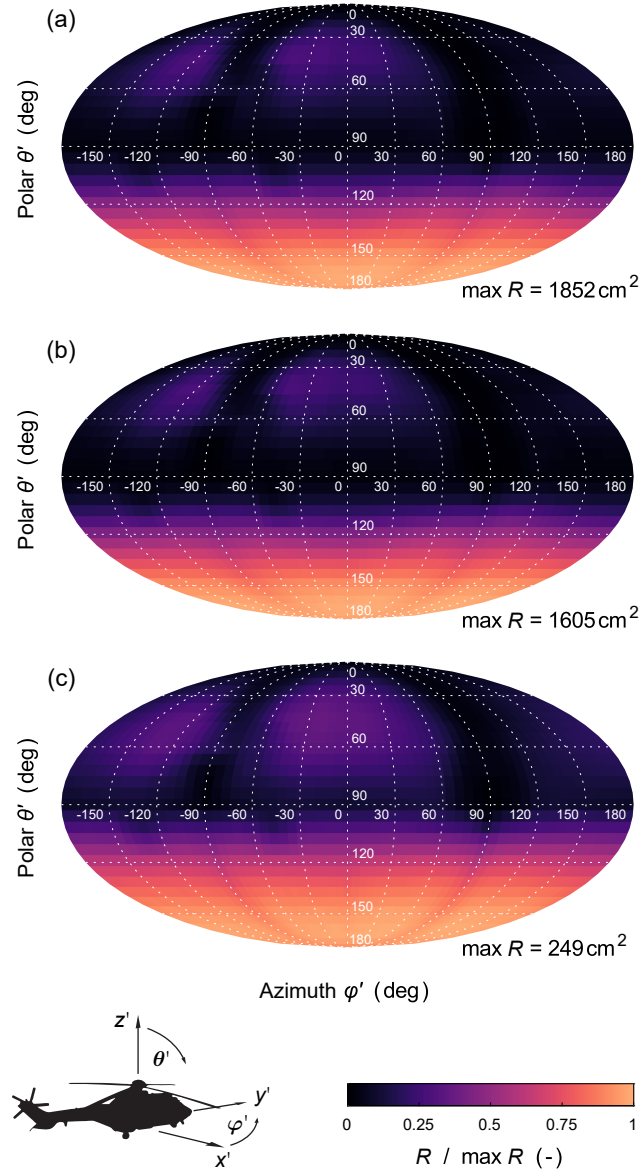

**Figure S3** Angular dispersion of the SAGRS system's instrument response  $R$  as a function of the polar angle  $\theta'$  and the azimuthal angle  $\varphi'$  with respect to the local non-inertial platform-fixed coordinate system  $x'$ - $y'$ - $z'$ . The angular dispersion was computed for a photon energy  $E_\gamma = 88 \text{ keV}$  and normalized by its maximum, i.e.  $R / \max R$  with  $\max R$  indicated in each graph. Three different spectral bands were evaluated: (a) Full-spectrum band ( $\mathcal{B}_{\text{tot}}$ ). (b) Full-energy band ( $\mathcal{B}_\gamma$ ). (c) Compton band ( $\mathcal{B}_C$ ). The angular dispersion graphs are interpolated on a regular  $6^\circ \times 6^\circ$  angular grid and displayed using the Mollweide projection.

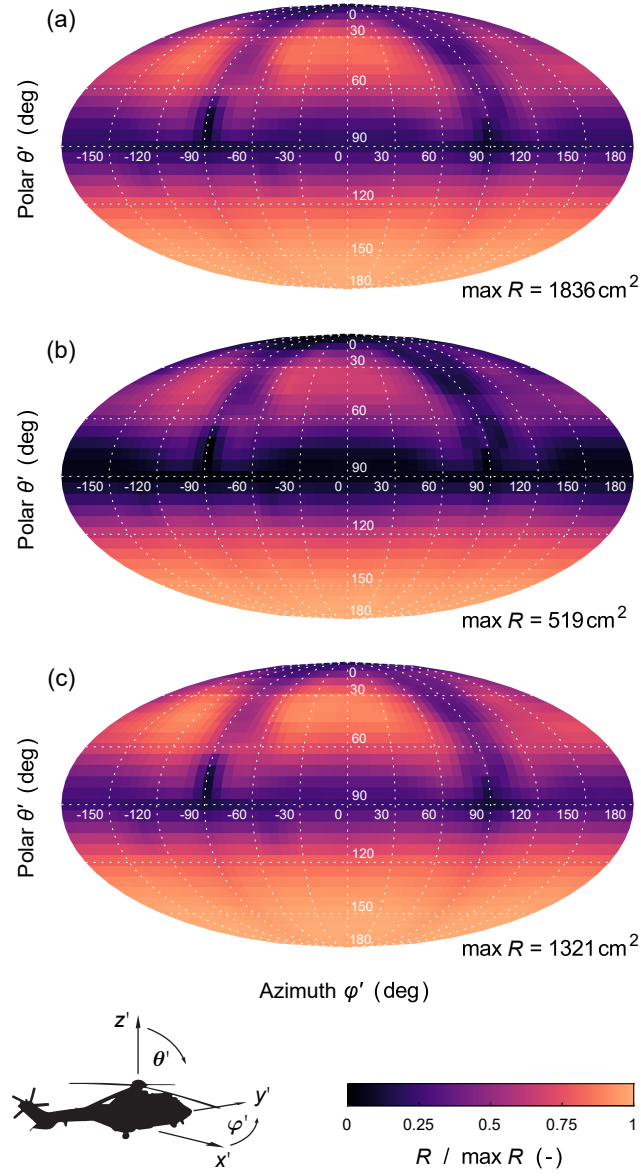

**Figure S4** Angular dispersion of the SAGRS system's instrument response  $R$  as a function of the polar angle  $\theta'$  and the azimuthal angle  $\varphi'$  with respect to the local non-inertial platform-fixed coordinate system  $x'-y'-z'$ . The angular dispersion was computed for a photon energy  $E_{\gamma} = 2615 \text{ keV}$  and normalized by its maximum, i.e.  $R / \max R$  with  $\max R$  indicated in each graph. Three different spectral bands were evaluated: (a) Full-spectrum band ( $\mathcal{B}_{\text{tot}}$ ). (b) Full-energy band ( $\mathcal{B}_{\gamma}$ ). (c) Compton band ( $\mathcal{B}_{\text{C}}$ ). The angular dispersion graphs are interpolated on a regular  $6^{\circ} \times 6^{\circ}$  angular grid and displayed using the Mollweide projection.

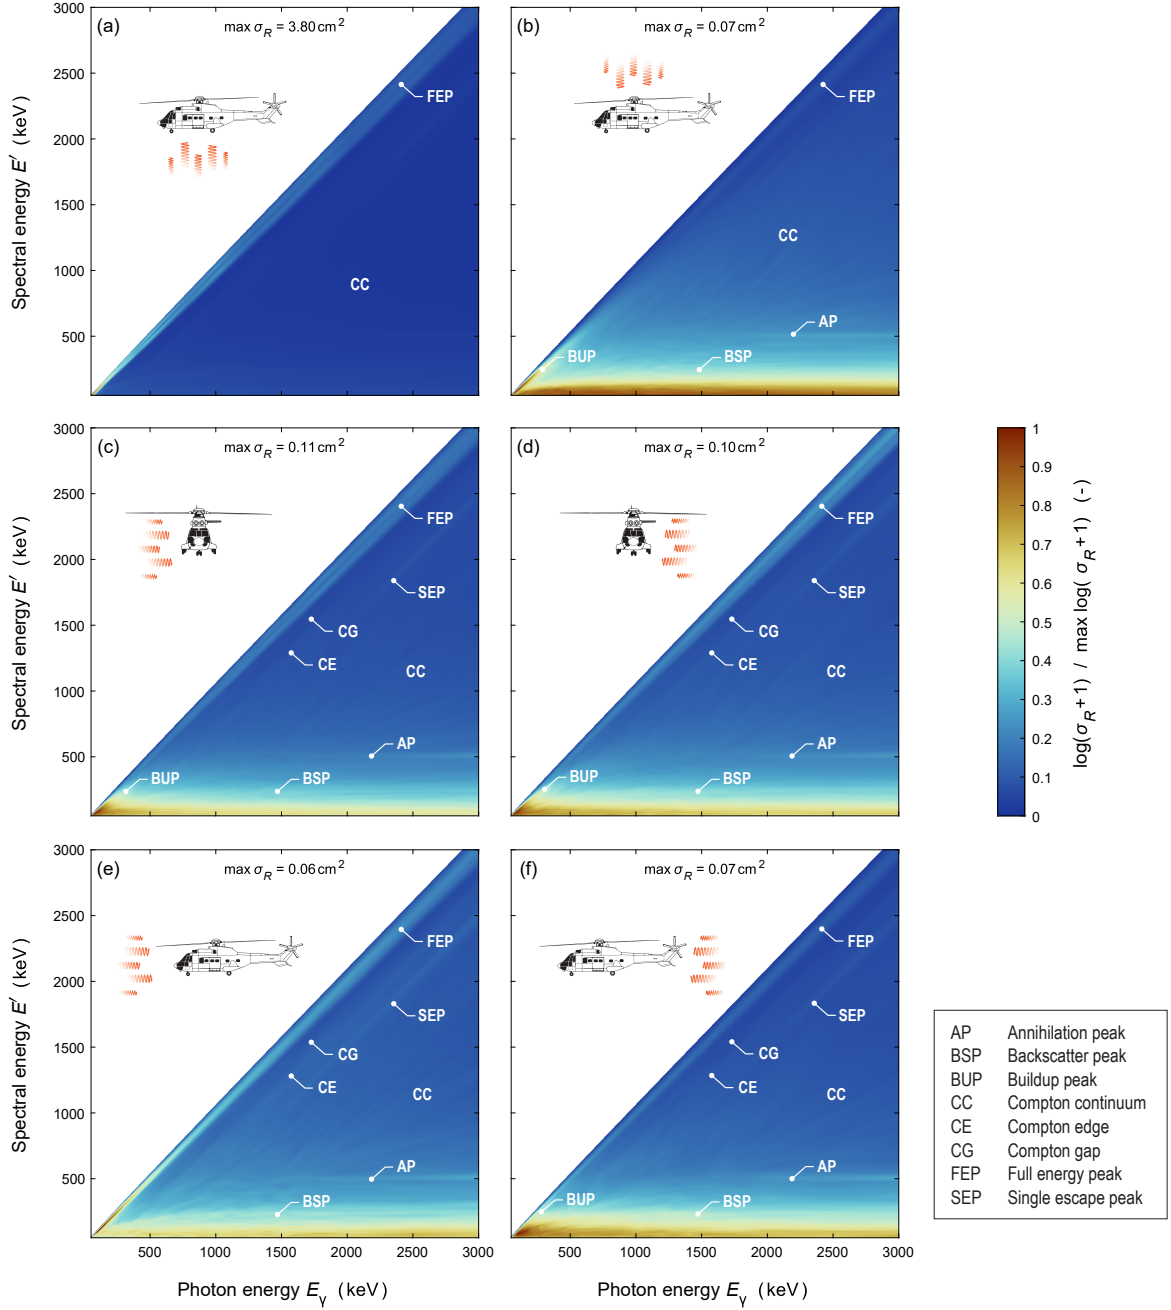

**Figure S5** Combined statistical and systematic uncertainties in the spectral dispersion of the SAGRS system's instrument response  $R$  characterized by the standard error of the mean  $\sigma_R$  as a function of the spectral energy  $E'$  and the gamma-ray energy  $E_\gamma$  with a constant spectral energy bin width  $\Delta E' \sim 3 \text{ keV}$ . The IRF was computed for the six cardinal incident directions (see also Fig. 1 in the main study): (a) Anti-normal ( $\theta' = 180^\circ$ ). (b) Normal ( $\theta' = 0^\circ$ ). (c) Starboard ( $\theta' = 90^\circ, \phi' = 0^\circ$ ). (d) Port ( $\theta' = 90^\circ, \phi' = 180^\circ$ ). (e) Forward ( $\theta' = 90^\circ, \phi' = 90^\circ$ ). (f) Backward ( $\theta' = 90^\circ, \phi' = -90^\circ$ ). Characteristic spectral features typical of inorganic scintillator responses are indicated [1, 2]. For visualization purposes, the IRF is constrained to the spectral energy range  $E' < E_\gamma + 3\sigma_E$  with  $\sigma_E$  being the spectral resolution standard deviation at  $E_\gamma$ . The line drawing of the AS332M1 helicopter displayed in the individual subfigures was adapted from Jetijones, CC BY 3.0, via Wikimedia Commons.



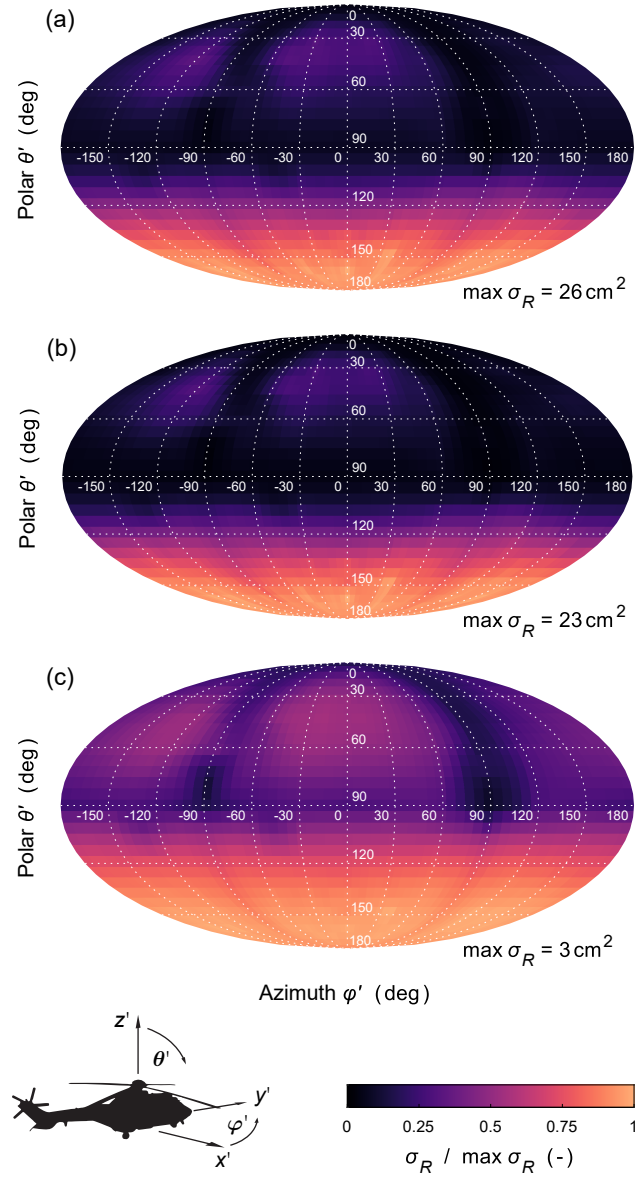

**Figure S6** Combined statistical and and systematic uncertainties in the angular dispersion of the SAGRS system's instrument response  $R$  characterized by the standard error of the mean  $\sigma_R$  as a function of the polar angle  $\theta'$  and the azimuthal angle  $\varphi'$  with respect to the local non-inertial platform-fixed coordinate system  $x'-y'-z'$ . The angular dispersion was computed for a photon energy  $E_\gamma = 88 \text{ keV}$  and normalized by its maximum, i.e.  $R / \max R$  with  $\max R$  indicated in each graph. Three different spectral bands were evaluated: (a) Full-spectrum band ( $\mathcal{B}_{\text{tot}}$ ). (b) Full-energy band ( $\mathcal{B}_\gamma$ ). (c) Compton band ( $\mathcal{B}_C$ ). The angular dispersion graphs are interpolated on a regular  $6^\circ \times 6^\circ$  angular grid and displayed using the Mollweide projection.

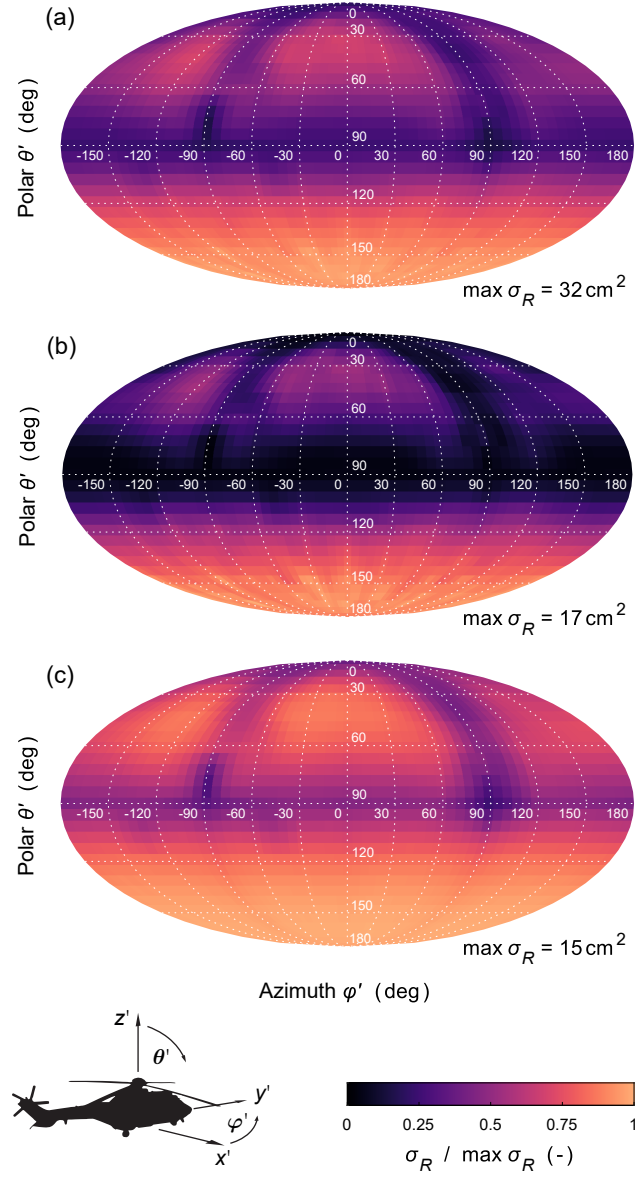

**Figure S7** Combined statistical and and systematic uncertainties in the angular dispersion of the SAGRS system's instrument response  $R$  characterized by the standard error of the mean  $\sigma_R$  as a function of the polar angle  $\theta'$  and the azimuthal angle  $\varphi'$  with respect to the local non-inertial platform-fixed coordinate system  $x'-y'-z'$ . The angular dispersion was computed for a photon energy  $E_\gamma = 662 \text{ keV}$  and normalized by its maximum, i.e.  $R/\max R$  with  $\max R$  indicated in each graph. Three different spectral bands were evaluated: (a) Full-spectrum band ( $\mathcal{B}_{\text{tot}}$ ). (b) Full-energy band ( $\mathcal{B}_\gamma$ ). (c) Compton band ( $\mathcal{B}_C$ ). The angular dispersion graphs are interpolated on a regular  $6^\circ \times 6^\circ$  angular grid and displayed using the Mollweide projection.

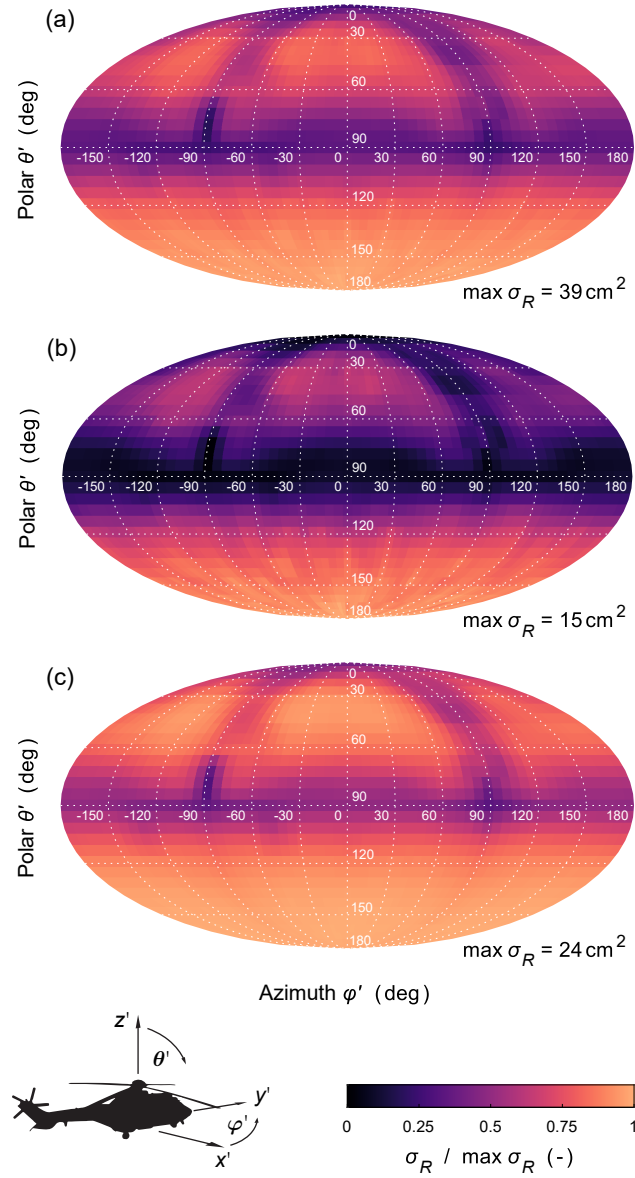

**Figure S8** Combined statistical and and systematic uncertainties in the angular dispersion of the SAGRS system's instrument response  $R$  characterized by the standard error of the mean  $\sigma_R$  as a function of the polar angle  $\theta'$  and the azimuthal angle  $\varphi'$  with respect to the local non-inertial platform-fixed coordinate system  $x'-y'-z'$ . The angular dispersion was computed for a photon energy  $E_\gamma = 2615 \text{ keV}$  and normalized by its maximum, i.e.  $R/\max R$  with  $\max R$  indicated in each graph. Three different spectral bands were evaluated: (a) Full-spectrum band ( $\mathcal{B}_{\text{tot}}$ ). (b) Full-energy band ( $\mathcal{B}_\gamma$ ). (c) Compton band ( $\mathcal{B}_C$ ). The angular dispersion graphs are interpolated on a regular  $6^\circ \times 6^\circ$  angular grid and displayed using the Mollweide projection.

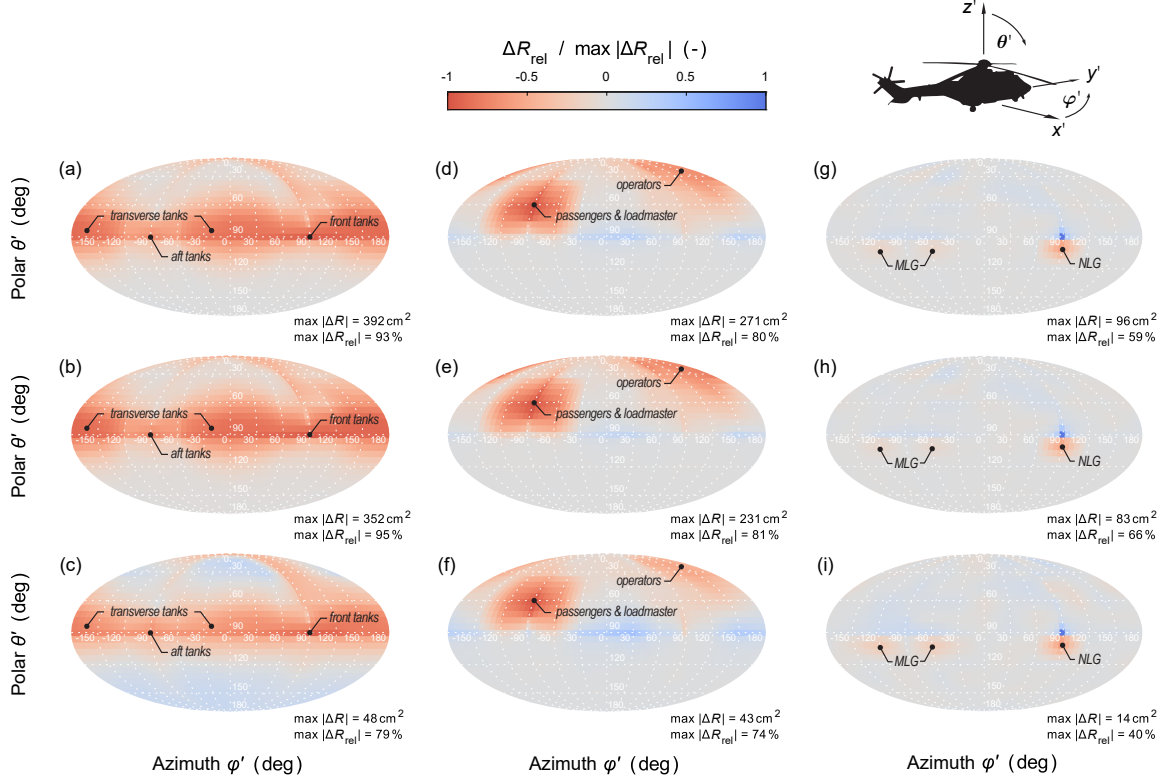

**Figure S9** Relative deviation in the angular dispersion of the SAGRS system's instrument response, defined as  $\Delta R_{\text{rel}} = \Delta R / R(\xi_0)$  with  $\Delta R := R(\xi_1) - R(\xi_0)$ , shown as a function of selected state variable changes  $\xi_0 \rightarrow \xi_1$ . Three perturbation scenarios are considered: (a–c) Fuel state from empty ( $\xi_0$ ) to full ( $\xi_1$ ). (d–f) Crew loading from unoccupied ( $\xi_0$ ) to maximum capacity ( $\xi_1$ ). (g–i) Landing gear deployment from retracted ( $\xi_0$ ) to extended ( $\xi_1$ ). All remaining parameters are kept at their fiducial value  $\xi_{\text{fid}}$  (see Section III A in the main study). For each state variable change, the instrument response is evaluated in three distinct spectral bands at a gamma-ray energy of  $E_\gamma = 88 \text{ keV}$ : (a, d, g) Full-spectrum band ( $\mathcal{B}_{\text{tot}}$ ). (b, e, h) Full-energy band ( $\mathcal{B}_\gamma$ ). (c, f, i) Compton band ( $\mathcal{B}_C$ ). All graphs are interpolated on a regular  $6^\circ \times 6^\circ$  angular grid and displayed using the Mollweide projection. Additionally, characteristic dynamic subsystems are annotated for reference, e.g. the main landing gear (MLG) and the nose landing gear (NLG) in the subfigures (g–i) (see also Appendix A in the main study).

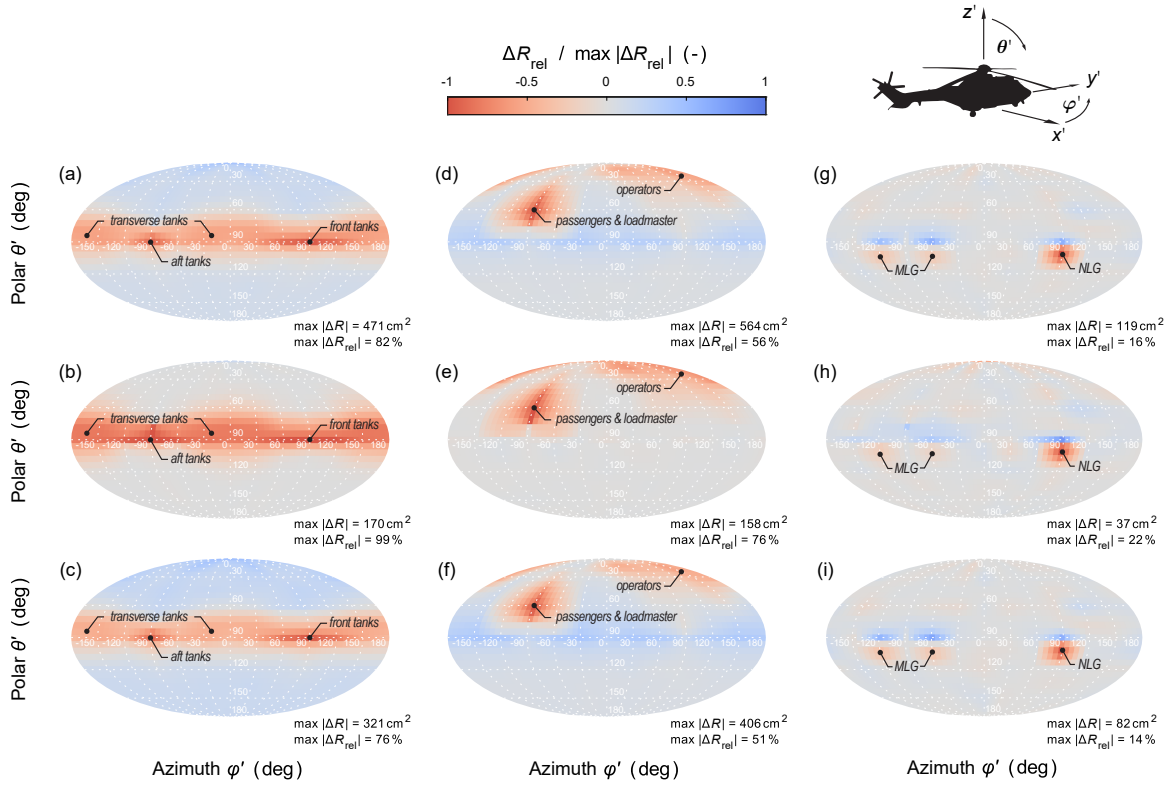

**Figure S10** Relative deviation in the angular dispersion of the SAGRS system's instrument response, defined as  $\Delta R_{\text{rel}} = \Delta R / R(\xi_0)$  with  $\Delta R := R(\xi_1) - R(\xi_0)$ , shown as a function of selected state variable changes  $\xi_0 \rightarrow \xi_1$ . Three perturbation scenarios are considered: (a–c) Fuel state from empty ( $\xi_0$ ) to full ( $\xi_1$ ). (d–f) Crew loading from unoccupied ( $\xi_0$ ) to maximum capacity ( $\xi_1$ ). (g–i) Landing gear deployment from retracted ( $\xi_0$ ) to extended ( $\xi_1$ ). All remaining parameters are kept at their fiducial value  $\xi_{\text{fid}}$  (see Section III A in the main study). For each state variable change, the instrument response is evaluated in three distinct spectral bands at a gamma-ray energy of  $E_\gamma = 2615 \text{ keV}$ : (a, d, g) Full-spectrum band ( $\mathcal{B}_{\text{tot}}$ ). (b, e, h) Full-energy band ( $\mathcal{B}_\gamma$ ). (c, f, i) Compton band ( $\mathcal{B}_C$ ). All graphs are interpolated on a regular  $6^\circ \times 6^\circ$  angular grid and displayed using the Mollweide projection. Additionally, characteristic dynamic subsystems are annotated for reference, e.g. the main landing gear (MLG) and the nose landing gear (NLG) in the subfigures (g–i) (see also Appendix A in the main study).

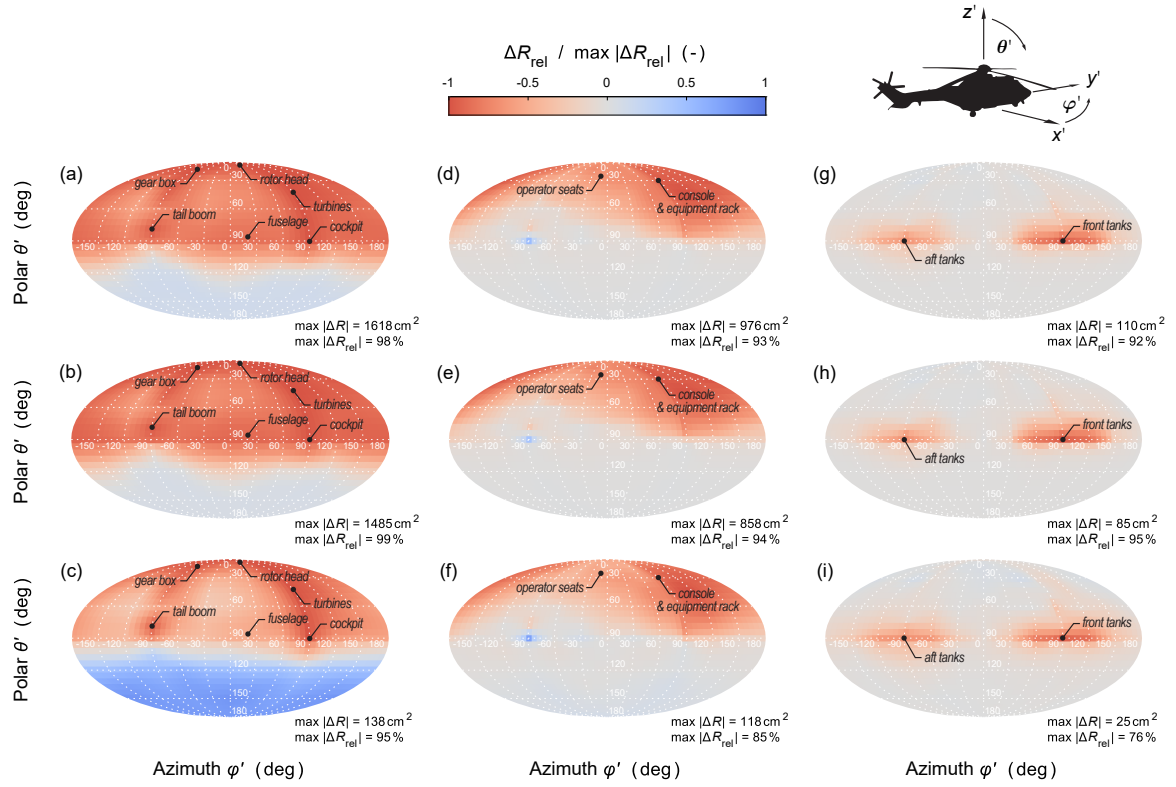

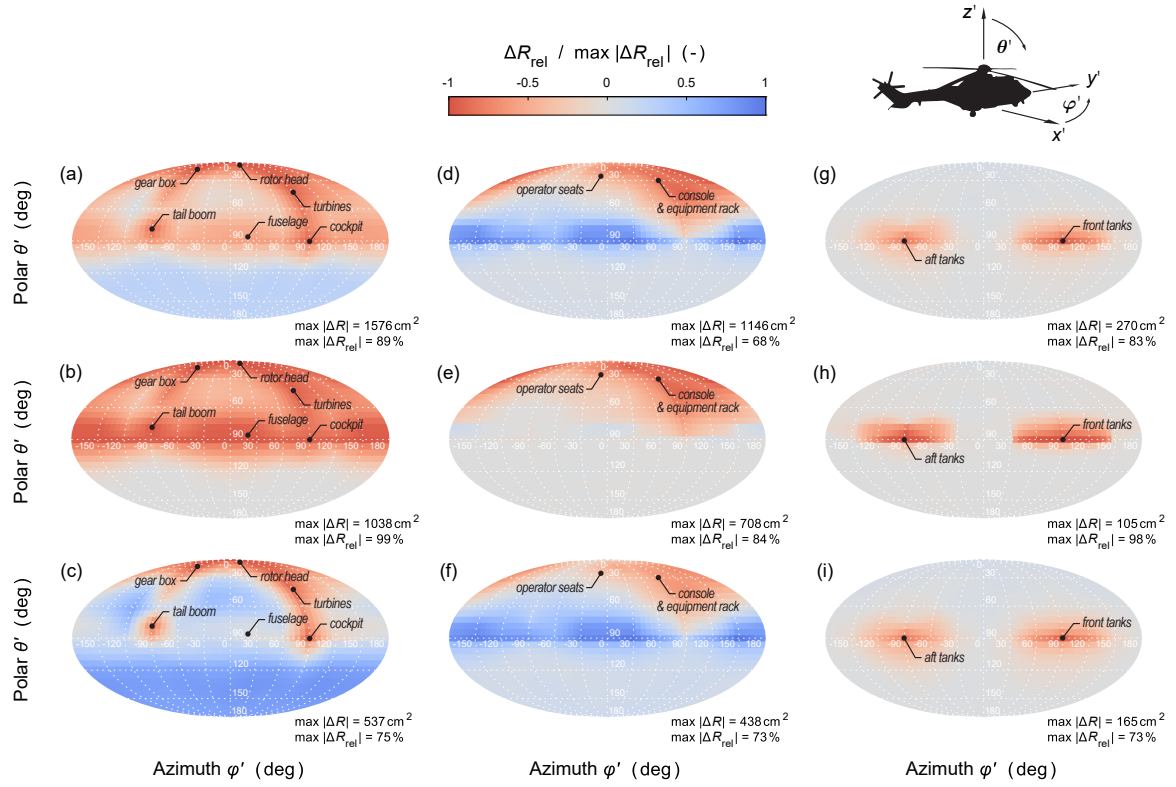



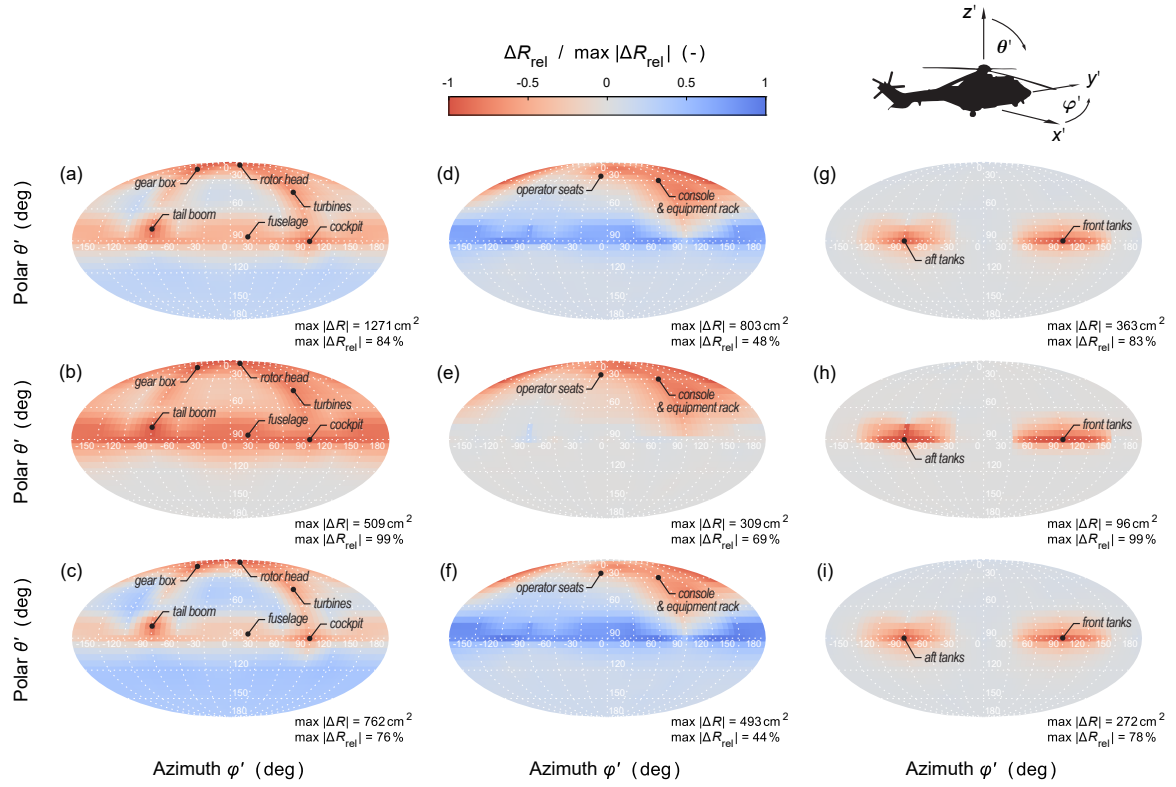



## Supplementary References

- [1] G. F. Knoll, Radiation Detection and Measurement, John Wiley & Sons, New York, USA, 2010.
- [2] D. Breitenmoser, Towards Monte Carlo Based Full Spectrum Modeling of Airborne Gamma-Ray Spectrometry Systems, Doctoral Thesis, ETH Zurich, 2024. doi:10.3929/ethz-b-000694094.
